# Supplementary material for: InfoNorm: Mutual Information Shaping of Normals for Sparse-View Reconstruction
Source: arXiv:2407.12661 source file (2024-07-17)
Supplement: Supplementary file 1 [file sam_ablation.tex]

\begin{figure*}[tb]
\centering
\includegraphics[width=1.0\linewidth]{supp_materials/sam_figure.pdf}
\caption{
}
\label{fig:sam_ablation}
\end{figure*}
