# Supplementary material for: InfoNorm: Mutual Information Shaping of Normals for Sparse-View Reconstruction
Source: arXiv:2407.12661 source file (2024-07-17)
Supplement: Supplementary file 3 [file training_iter.tex]

%\begin{table}[tb]
\begin{wraptable}{r}{0.32\textwidth}
%\vspace{-34pt}
%\vspace{-20pt}
\caption{Traning iters.}
\centering
\resizebox{0.25\textwidth}{!}{
\begin{tabular}{@{}lc@{}}
    \toprule
    Method & Iters\\
    \midrule
    
    NeuS$^+$  & 160000 \\
    VolSDF$^+$ & 150000 \\
    
    GeoNeuS$^+$ & 150000 \\
    $I^2$-SDF$^+$ & 150000 \\

    NeuRIS$^+$ & 160000 \\
    MonoSDF$^+$ & 100000 \\

    Neuralangelo$^+$ & 150000 \\
    
  \bottomrule
\end{tabular}
}
%\vspace{-35pt}
\label{tab:training_iter}
%\end{table}
\end{wraptable}
